# Supplementary material for: Trustworthy Reinforcement Learning Against Intrinsic Vulnerabilities: Robustness, Safety, and Generalizability
Source: arXiv:2209.08025 source file (2022-09-16)
Supplement: Supplementary file 1 [file appendix.tex]

\appendix
\section{Notation System}
\label{append:notations}

  \subsection{Notation Convention}
  \begin{enumerate}
    \item Function: lowercase letter, e.g. $f$, $f(\cdot)$ 
    \item Scalar: lowercase letter, e.g. $x$
    \item Random variable: uppercase letter, e.g. $X$
    \item Matrix:  uppercase letter, e.g. $K$
    \item Common number set: Upper case double letter, e.g. $\mathbb R$ 
    \item Context-based set: Upper case script letter, e.g. $\mathcal A$ 
  \end{enumerate}
  
  \subsection{Alphabet Letter}
  %\begin{table}[h!]
  
  \ding{rerank them by alphabetical order}
  \begin{longtable}{ |l|p{6cm}|p{6cm}|  }
     %\hline
     %\multicolumn{3}{|c|}{Alphabet Letter} \\
     \hline
     Symbol& Designation &Note/Example\\
     \hline
     %%%----- alphabet letters ------
     $\mathbb{1} (\cdot)$   & Indicator function    & \\
     \hline
      $d $   & dimension of input variable   & \\
     \hline
     $\mathcal D$   & dataset   & \\
     \hline
     $\mathbb E[\cdot]$   & Expectation    & -\\
     \hline
     $\mathbb E_p [\cdot]$   & Expectation taken with pdf $p$    & -\\
     \hline
      $f, f (\cdot)$   & Mapping representation of system, relating input to output  & \\
       \hline
         $\mathcal{GP}(m, K) $   & Gaussian process with mean $m$ and covariance $K$    & \\
     \hline
     $n$   & Number of samples    & \\
     \hline
     $\mathcal{N}(\mu, \sigma^2I) $   & Normal distribution with mean $\mu$ and variance $\sigma^2$    & \\
     \hline
     $p$   & Probability distribution (original)    & \\
     \hline
     $P (\cdot)$   & Probability    & \\
     \hline
     $q$   & Probability distribution (biasing/proposal)    & \\
     \hline
     $\mathcal Q$   & Set of proposal distributions    & \\
     \hline
     $\mathbb{R} $   & Real set    & \\
     \hline
     $\text{Std}(\cdot) $   & Standard Deviation    & \\
     \hline
     $\text{Var}(\cdot) $   & Variance    & \\
     \hline
     $x$   & A generic variable representing input to system & The default is $x = [x_1, \cdots, x_d]$ \\
     \hline
     $X$   & Random variable representation of $x$ & $X^{(1)}, \cdots, X^{(n)}$ means $n$ samples of $X$. Each sample $X^{(i)} = [X_1^{(i)}, \cdots, X_d^{(i)}]$, for $i=1, 2, \cdots, n$. \\
     \hline
     $y$   & Variable representing output of the system    & $y = f(x)$\\
     \hline
     $Y$   & Random variable representation of $y$    & $Y = f(X)$\\
     \hline
     $s$   & a state    & \\
     \hline
      $s^\prime$   & the next state    & \\
     \hline
     $\mathcal{S}$   & state space    & $s \in \mathcal{S}$\\
     \hline 
     $a$   & an action   & \\
     \hline
     $\mathcal{A}$   & action space    & $a \in \mathcal{A}$\\
     \hline 
      $r(s,a)$   & expected immediate reward from state $s$ after action $a$    & \\
     \hline
     $G_t$   & return (discounted cumulative reward) following time t  & $G = \sum_{t} \gamma^t r_t $\\
     \hline 
      $p(s^\prime | s, a)$   & probability of transition to state $s^\prime$, from state $s$ taking action $a$  &\\
     \hline 
       $J(\theta)$   & performance measure for the policy $\pi_\theta$  &\\
     \hline
      $L$   & loss function  &\\
      
     \hline
     
    \end{longtable}
    %\end{table}
  
  \subsection{Greek Letter}
  \begin{table}[h!]
      \begin{tabular}{ |l|p{6cm}|p{6cm}|  }
     \hline
     Symbol& Designation &Note/Example\\
     \hline
     %%%----- greek letters ------
     $\epsilon$   & Small positive scalar   & (epsilon or varepsilon)\\
     \hline
     $\theta$   & Parameter of system approximation & -\\
     \hline
      $\Theta$   & Set of possible parameters & $\theta \in \Theta$\\
     \hline
     $\mu$   & Mean & -\\
     \hline
     $\mu_X$   & Mean of random variable $X$   & -\\
     \hline
     $\sigma$   & (Unbiased) standard deviation   & $\sigma^2$: (Unbiased) Variance\\
     \hline
      $\sigma_X$   & (Unbiased) standard deviation of r.v. $X$ & $\sigma_X^2$: (Unbiased) variance of $X$\\
     \hline
      $\gamma$   & discount factor of reward & $R = \sum_{t} \gamma^t r_t $\\
     \hline
        $\tau$   & experience of an episode & $\tau = \{s_0, a_0, \dots, s_T, a_T \} $\\
     \hline
    $\pi$   & policy of an agent & $\pi(a | s)$: stochastic policy ; $\pi(s)$: deterministic policy\\
     \hline
    \end{tabular}
    \end{table}

\section{Adversarial Attacks in RL}

\subsection{Variants of MDPs}

\ding{we may keep this section but need to augment it with CMDP and contextual MDP}

\begin{definition}[SA-MDP]

\end{definition}

\begin{definition}[PR-MDP~\cite{tessler2019action}]
\label{def:pr-mdp}
Let $\pi$ and $\bar\pi$ be policies of an agent and an adversary. Let $\alpha\in[0,1]$, we define the probabilistic joint policy $\pi_{P, \alpha}^{\mathrm{mix}}(\pi, \bar{\pi})$ as $\pi_{P, \alpha}^{\operatorname{mix}}(a \mid
\text { s) } \equiv(1-\alpha) \pi(a \mid s)+\alpha \bar{\pi}(a \mid s), \forall s \in \mathcal{S}$.
The value of the policy $\pi$ is defined by $v_{P, \alpha}^{\pi}=\min _{\bar{\pi} \in \Pi} \mathbb{E}^{\pi_{P, \alpha}^{\operatorname{mix}}(\pi, \bar{\pi})}\left[\sum_{t} \gamma^{t} r\left(s_{t}, a_{t}\right)\right]$, where $a_{t} \sim \pi_{P, \alpha}^{\operatorname{mix}}\left(\pi\left(s_{t}\right), \bar{\pi}\left(s_{t}\right)\right)$.
The optimal probabilistic robust policy is the optimal policy of the PR-MDP
\begin{align}
    \pi_{P, \alpha}^{*} \in \underset{\pi \in \mathcal{P}(\Pi)}{\arg \max } \min _{\bar{\pi} \in \Pi} \mathbb{E}^{\pi_{P, \alpha}^{\operatorname{mix}}(\pi, \bar{\pi})}\left[\sum_{t} \gamma^{t} r\left(s_{t}, a_{t}\right)\right].
\end{align}
\end{definition}
\begin{definition}[NR-MDP~\cite{tessler2019action}]
\label{def:nr-mdp}
Let $\pi$ and $\bar\pi$ be policies of an agent and an adversary. Let $\alpha\in[0,1]$, we define the noisy joint policy $\pi_{N, \alpha}^{\operatorname{mix}}(\pi, \bar{\pi})$ as $\pi_{N, \alpha}^{\operatorname{mix}}(\mathbf{a} \mid \mathbf{s}) \equiv \mathbb{E}_{\mathbf{b} \sim \pi(\cdot \mid s)}\left[\mathbb{1}_{\mathbf{a}=(1-\alpha) \mathbf{b}+\alpha \overline{\mathbf{b}}}\right],\forall s \in \mathcal{S}, \mathbf{a} \in \mathcal{A}$.
The value of the policy $\pi$ is defined by $v_{N, \alpha}^{\pi}=\min _{\bar{\pi} \in \Pi} \mathbb{E}^{\pi_{N, \alpha}^{m, \alpha}(\pi, \bar{\pi})}\left[\sum_{t} \gamma^{t} r\left(\mathbf{s}_{t}, \mathbf{a}_{t}\right)\right]$, where $\mathbf{a}_{t} \sim \pi_{N, \alpha}^{\operatorname{mix}}\left(\pi\left(\mathbf{s}_{t}\right), \bar{\pi}\left(\mathbf{s}_{t}\right)\right)$.
The optimal noisy robust policy is the optimal policy of the NR-MDP
\begin{align}
    \pi_{N, \alpha}^{*} \in \underset{\pi \in \mathcal{P}(\Pi)}{\arg \max } \min _{\bar{\pi} \in \Pi} \mathbb{E}^{\pi_{N, \alpha}^{\operatorname{mix}(\pi, \bar{\pi})}}\left[\sum_{t} \gamma^{t} r\left(\mathbf{s}_{t}, \mathbf{a}_{t}\right)\right].
\end{align}
\end{definition}
\begin{definition}[CRMDP~\cite{everitt2017reinforcement}]
\label{def:cr-mdp}
A corrupt reward MDP (CRMDP) is defined by a tuple $(\cal S,\cal A, \cal R, P, \dot{ R},C,\hat{R})$.
In the environment with potentially corrupted reward, we use a \textit{dot} to represent the \textit{true} signal and a \textit{hat} to represent the \textit{observed} counterpart.
Specifically, we use $\dot{\mathcal{R}},\hat{\mathcal{R}},\mathcal{R}\subseteq \bb R$ to denote the finite reward sets, and these three sets are equivalent.
$\dot{R}:\cal S\times \cal A \rightarrow \hat{\cal R}$ is the true reward function and $C:\cal S\times \dot{\cal R}\rightarrow \hat{\cal R}$ is the reward corruption function.
We express the state dependency of the corruption function as a superscript: $C_s(\hat r):=C(s,\hat r)$.
The observed reward function is thus $\hat R: \cal S\times \cal A\rightarrow \hat{\cal R}$ defined as $\hat R(s):=C_s(\dot{R}(s))$.
\end{definition}

\subsection{Detailed Categorization of Threat Models}
\label{append:attack-threat-model}

\subsection{Backdoors in DRL}

In backdoor (trojan) attacks~\cite{gu2017badnets,chen2017targeted}, the adversary can inject backdoors to elicit unanticipated behavior from a model that works properly on benign input. 
Recent work demonstrate the existence of backdoor attacks in RL settings, \eg,
black-box trojan attacks in partially observable environments against LSTM policy networks~\cite{yang2020backdoor},
white-box and black-box attacks utilizing data poisoning and reward hacking under different combinations of threat models~\cite{kiourti2020trojdrl},
adversary agent in a competitive RL setup that can trigger the backdoor of the victim agent with its own action~\cite{wang2021backdoorl},
as well as backdoors in traffic congestion control systems with triggers designed based on well-established principles of traffic physics~\cite{wang2020stop}.
As evaluated in these works, existing defense mechanisms against trojan attacks in classification tasks (\eg, Fine-Pruning~\cite{liu2018fine} and Neural Cleanses~\cite{wang2019neural}) are ineffective against these backdoor attacks in DRL, which motivate the development of more targeted and advanced defense mechanisms for improved robustness.
% Yang \etal~\cite{yang2020backdoor} developed a black-box trojan attack in partially observable environments against LSTM policy networks.
% Under this attack, the agent will switch to the malicious policy after observing the trigger at certain time steps. 
% Kiourti \etal~\cite{kiourti2020trojdrl} consider different combinations of threat models and present algorithms for both data poisoning and reward hacking in targeted and untargeted attacks, implemented as open-loop attacks.

\subsection{Policy Poisoning}

Online RL~\cite{zhang2021robustpg}, Offline RL~\cite{ma2019policy}, multi-stage episodic RL~\cite{lykouris2019corruption}
